# Supplementary material for: Cosmological Asymptotics in Higher-Order Gravity Theories
Source: arXiv:1706.01360 source file (2017-06-05)
Supplement: Supplementary file 3 [file AppendixTemplate.tex]

% Appendix Template

\chapter{Appendix Title Here} % Main appendix title

\label{AppendixX} % Change X to a consecutive letter; for referencing this appendix elsewhere, use \ref{AppendixX}

\lhead{Appendix X. \emph{Appendix Title Here}} % Change X to a consecutive letter; this is for the header on each page - perhaps a shortened title

Write your Appendix content here.
